# Supplementary material for: Memorisation and forgetting in a learning Hopfield neural network: bifurcation mechanisms, attractors and basins
Source: arXiv:2508.10765 ancillary file (2026-02-15)
Supplement: Supplementary file 1 [file EJNB_NN_bif_mech_SN.pdf]

# Memorisation and forgetting in a learning Hopfield neural network: bifurcation mechanisms, attractors and basins

## SUPPLEMENTARY NOTE

Adam E. Essex,<sup>1, a)</sup> Natalia B. Janson,<sup>1, b)</sup> Rachel A. Norris,<sup>1</sup> and Alexander G. Balanov<sup>2, c)</sup>

<sup>1)</sup>*Department of Mathematical Sciences, Loughborough University, Loughborough LE11 3TU, UK*

<sup>2)</sup>*Department of Physics, Loughborough University, Loughborough LE11 3TU, UK*

### CONTENTS

|                                                                                                    |   |
|----------------------------------------------------------------------------------------------------|---|
| <b>S-I. Visualising energy landscape for a Hopfield network with Heaviside activation function</b> | 1 |
| <b>S-II. Training data for learning Hopfield network</b>                                           | 1 |
| <b>S-III. Hopfield network in alternative form</b>                                                 | 2 |
| <b>S-IV. Appendix of Tables</b>                                                                    | 5 |

### S-I. VISUALISING ENERGY LANDSCAPE FOR A HOPFIELD NETWORK WITH HEAVISIDE ACTIVATION FUNCTION

In the main paper we analyse Hopfield neural network (NN) in the form of Ref.<sup>S1</sup>, which reads:

$$\frac{dx_i}{dt} = -x_i + g \sum_{j=1}^N F(\omega_{ij}) F(x_j) + AI_i(t), \quad (S1)$$

$$\frac{d\omega_{ij}}{dt} = \frac{1}{B_{ij}} (-\omega_{ij} + F(x_i) F(x_j)). \quad (S2)$$

Equations (S1)–(S2) are identical to (1)–(2). Here  $x_i(t)$ ,  $i=1, \dots, N$ , is the state of  $i^{\text{th}}$  neuron at time  $t$ ;  $\omega_{ij}(t)$  is the instantaneous strength of coupling (connection weight) between  $i^{\text{th}}$  and  $j^{\text{th}}$  neurons with  $\omega_{ij} = \omega_{ji}$ ; and  $I_i(t)$  represents external input to  $i^{\text{th}}$  neuron, which is used for training the network.

To visualise energy landscape of this NN, assume that activation function  $F$  takes the form of Heaviside step function,

$$F(x) = \begin{cases} -1, & x < 0 \\ 1, & x \geq 0 \end{cases} \quad (S3)$$

since in this case Eq. (S1) can be rewritten as

$$\frac{dx_i}{dt} = -\frac{\partial V}{\partial x_i} \quad (S4)$$

with

$$V = \sum_{i=1}^N \left[ \frac{(x_i - AI_i(t))^2}{2} - gx_i \sum_{j=1}^N F(\omega_{ij}) F(x_j) \right]. \quad (S5)$$

The scalar function  $V=V(\mathbf{x}, t)$  is an instantaneous energy landscape for the neural activity, which allows one to interpret Eqs. (S1)–(S2) as a model describing the motion of a particle with location  $\mathbf{x}(t)$  in the landscape  $V$ .

For the same value of  $N=81$  as in Ref.<sup>S1</sup>, we visualise  $V$  after training of (S1)–(S2) is completed at  $t=6000$  and the values of  $\omega_{ij}$  are fixed. Post-training, the NN model is obtained by setting  $A=0$  in (S1):

$$\frac{dx_i}{dt} = -x_i + g \sum_{j=1}^N F(\omega_{ij}) F(x_j). \quad (S6)$$

Equation (S6) describes the NN during memory retrieval, when the system is launched from initial conditions equal to a vector coding the pattern that needs to be recognised as belonging to a certain category. This is achieved by the state  $\mathbf{x}$  of (S6) converging to the respective attractor.

Visualising a scalar function  $V$  of 81 variables in full with conventional approaches is impossible. However, we can visualise  $V$  on a *two-dimensional* cross-section of the  $N$ -dimensional phase space of the NN. Consider slicing the 81-dimensional space of (S6) by 79 mutually orthogonal hyperplanes defined as  $x_3=\hat{x}_3, \dots, x_{81}=\hat{x}_{81}$ , where  $\hat{\mathbf{x}}$  is the location of one of the stable fixed points of (S6). These 79 hyperplanes intersect along a two-dimensional plane  $(x_1, x_2)$ , which represents the *secant* plane of the phase space of the NN.

The function  $V$  on two different cross-sections, corresponding to two different secant planes going through two different fixed-point attractors, is shown in Fig. S1(a)–(b). The respective attractors, as well as others not illustrated, are formed as a result of learning by (S1)–(S2) from the training signal  $\mathbf{I}(t)$  constructed from six vectors of Set 1 specified in Tabs. S1–S2, as described in Sec. S-II and in Sec. III of the main paper.

Coloured surfaces in Fig. S1 show  $V$  in two different two-dimensional cross-sections of the phase space, and filled circles show locations  $(x_1, x_2)$  of the attractors  $\hat{\mathbf{x}}$  used to specify the respective cross-sections. Both attractors lie exactly at the bottom of each well, supporting the idea that  $V$  represents a potential energy for  $\mathbf{x}$ .

### S-II. TRAINING DATA FOR LEARNING HOPFIELD NETWORK

Below we describe training data applied to the Hopfield NN (S1)–(S2) (also (1)–(2)). Most results were obtained for  $N=81$  as in Ref.<sup>S1</sup>, hence the input  $\mathbf{I}(t)$  was constructed from

<sup>a)</sup>E-mail: A.Essex@lboro.ac.uk

<sup>b)</sup>E-mail: N.B.Janson@lboro.ac.uk

<sup>c)</sup>E-mail: A.Balanov@lboro.ac.uk

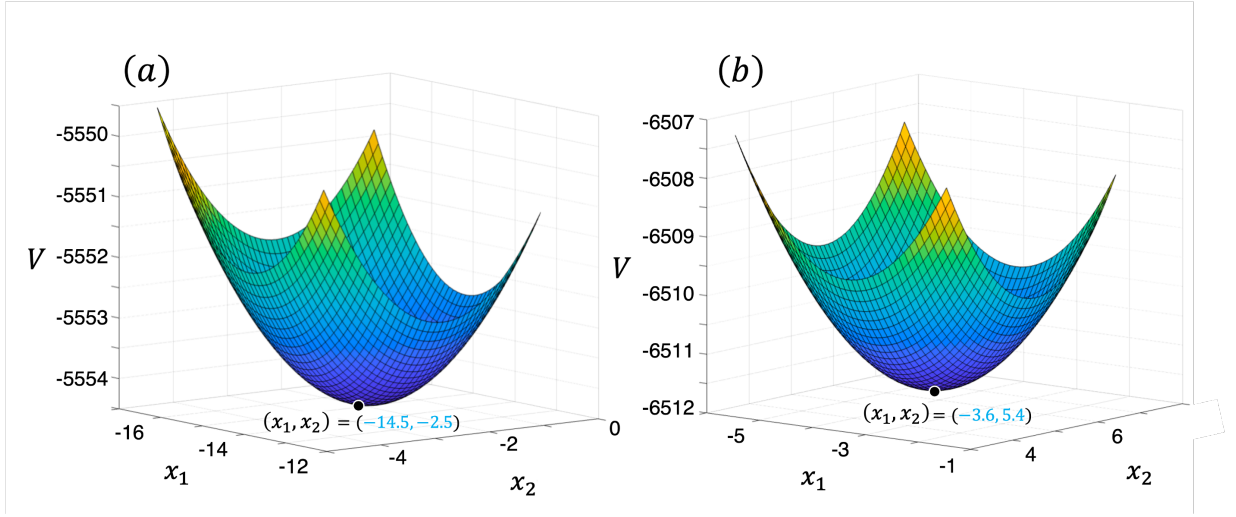

FIG. S1. Energy landscape  $V(\mathbf{x}, t)$ , specified by (S5), for the NN (S6) with  $N=81$  and  $\omega_{ij}$  set to the values achieved by (S1)–(S2) after it learns from the training signal  $\mathbf{I}(t)$  formed from six vectors  $\mathbf{I}^k$  of Set 1 (Tabs. S1–S2). In (a) and (b) the landscape  $V$  is shown on two different cross-sections of 81-dimensional phase space of (S6) defined by  $x_3=\hat{x}_3, \dots, x_{81}=\hat{x}_{81}$ , where  $\hat{\mathbf{x}}$  is the location of one of the attracting fixed points in (S6). Filled circles indicate locations of two attractors used to define the cross-sections, which lie at the bottom of each well, respectively.

six 81-dimensional vectors representing certain patterns. Following Ref.<sup>S1</sup>, each component of an input vector was chosen at random from the set  $\{-1, +1\}$  with equal probability, and each draw was statistically independent of all others. This way, for each of the two sets of training data Set 1 and Set 2, six vectors were generated, which are provided in Tabs. S1–S2. From the vectors of each of this set, a training signal lasting 6000 time units was generated, as discussed in in Sec. III of the main paper and illustrated in Fig. 1. Despite the equivalence of procedures leading to the two training sets, the outcomes of learning from them were different. Namely, with Set 1, only five out of six patterns were learnt, whereas with Set 2 all six patterns were learnt successfully.

In addition to the 81-neuron network, the main paper presents some results illustrating how system (1)–(2) learns with  $N=3$ . For this system, a set of three training vectors were generated, as described above (see Tab. S3). For this smaller model, only three vectors (coding some unspecified patterns) were used rather than six due to the smaller size of the network limiting its capacity to store memories.

### S–III. HOPFIELD NETWORK IN ALTERNATIVE FORM

The leading results presented in the main paper were obtained for the original form of the Hopfield network<sup>S1</sup> described by Eqs. (1)–(2). However, we show that conclusions drawn from these results also hold for an alternative, simpler form of the Hopfield network in which the weights  $\omega_{ij}$  appear

linearly in the equation describing neural activity as follows:

$$\frac{dx_i}{dt} = -x_i + g \sum_{j=1}^N \omega_{ij} F(x_j) + A I_i(t), \quad (\text{S7})$$

$$\frac{d\omega_{ij}}{dt} = \frac{1}{B_{ij}} (-\omega_{ij} + F(x_i) F(x_j)), \quad (\text{S8})$$

where Eq. (S8) for  $\omega_{ij}$  is the same as (S2). Despite this alteration in the nature of the coupling, we find that (S7)–(S8) behave in a qualitatively the same manner as (S1)–(S2). In this Section we illustrate this similarity by revealing attractors and their basins of (S7)–(S8) after this NN was trained following the same protocol as (S1)–(S2) (or (1)–(2)) with the training signal formed from Set 1 from Tabs. S1–S2.

As for (S1)–(S2), the training signal  $\mathbf{I}(t)$  for this network was generated by allowing each of six vectors  $\mathbf{I}^k$ ,  $k = 1, \dots, 6$ , from the Set 1 to consecutively stay constant during 12 time units, thus forming 81 telegraph signals shown in Fig. 1. Each of the resultant 81 segments were repeated many times until the total duration of the training signal reached 6000 time units. For this simulation the following parameters were used:  $A=30$ ,  $g=0.3$ ,  $B=300$ . Also, initial conditions (ICs) for  $x_i$  and  $\omega_{ij}$  were the same as for (S1)–(S2). After 6000 time units, simulations of (S7)–(S8) were stopped. The weights  $\omega_{ij}$  were fixed at their values at the end of training and substituted into the autonomous NN describing pattern recognition,

$$\frac{dx_i}{dt} = -x_i + g \sum_{j=1}^N \omega_{ij} F(x_j), \quad (\text{S9})$$

which is equivalent to (S7) with  $A=0$ .

In the post-training NN (S9), all attracting fixed points were revealed and visualized in projections onto the  $(x_1, x_2)$  plane. To associate specific attractors with applied vectors  $\mathbf{I}^k$ , we set

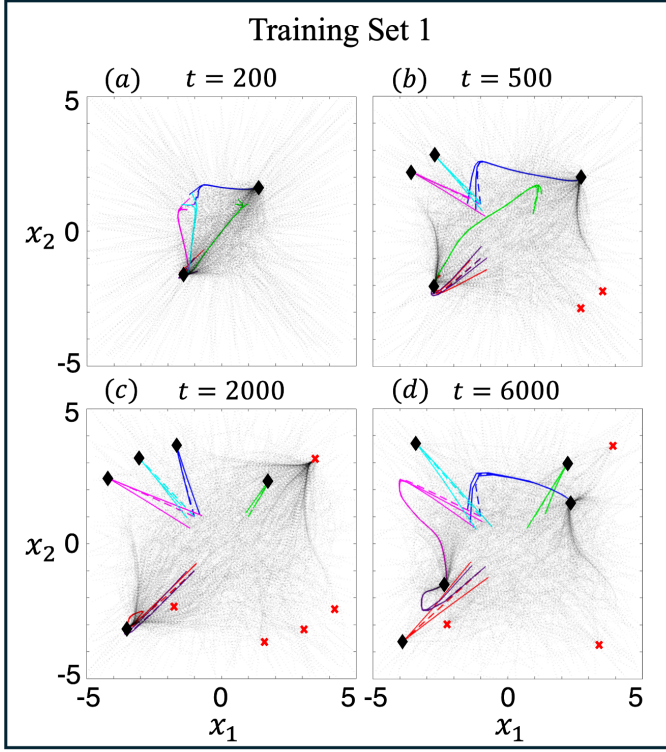

FIG. S2. Projection of the phase portraits of the NN (S9) with  $N=81$  on the plane  $(x_1, x_2)$  at various stages of learning (described by  $t$ ) in its counterpart system (S7)–(S8). The weights  $\omega_{ij}$  in (S9) were fixed at the values they take in (S7)–(S8) at times (a)  $t=200$ , (b)  $t=500$ , (c)  $t=2000$ , and (d)  $t=6000$  (the end of learning). The NN (S7)–(S8) was trained with  $\mathbf{I}(t)$  formed from the training Set 1 from Tabs. S1–S2. Black diamonds represent attractors coding true memories of input vectors  $\mathbf{I}^k$ , red crosses indicate spurious attractors not associated with any  $\mathbf{I}^k$ . Dashed coloured lines represent phase trajectories from Type 1 ICs (six in total, one for each pattern), solid coloured lines represent phase trajectories from Type 2 ICs (12 total, two for each  $\mathbf{I}^k$ ) and dashed grey lines represent phase trajectories from Type 3 ICs (1000 in total).

ICs to be equal to each of these vectors (Type 1 ICs as described in Sec. III) and also to the points belonging to their small vicinities (Type 2 ICs as described in Sec. III), and observe the attractor to which the respective phase trajectories converge. We perform this analysis at various stages of training by memorizing the weights  $\omega_{ij}(t)$  in (S7)–(S8) at several values of time  $t$ , 200, 500, 2000 and 6000, and then launching (S9) with each of these memorized sets of  $\omega_{ij}$  from the collection of ICs described above. This is illustrated in Fig. S2, which shows the projections onto  $(x_1, x_2)$  plane of all attractor fixed points and of phase trajectories.

Namely, in Fig. S2(d) after the full training is completed at  $t=6000$ , five black diamonds show attractors representing true memories of applied patterns (vectors  $\mathbf{I}^k$ ), which can be discovered by observing that these points attract phase trajectories launched from ICs equal to the respective vectors  $\mathbf{I}^k$  (Type 1, colored dashed lines) and from their small vicinities (Type 2, colored solid lines). Note, that out of the five true attractors/memories, one is associated with two different  $\mathbf{I}^k$ s

(see purple and violet lines converging to the same diamond).

To reveal all available attractors, including those linked to true and spurious memories, we launch (S9) from 1000 randomly chosen ICs uniformly distributed in the phase space (Type 3 ICs as described in Sec. III). This way, we revealed spurious memories, i.e. attractors (red crosses) not associated with any input vector  $\mathbf{I}^k$ . The phase trajectories launched from such ICs are shown by dashed grey lines in Fig. S2(d).

We can see from Fig. S2 that the number and the location of memories developed at the end of learning in the alternative form (S7)–(S8) of the NN match almost exactly those for the original model (S1)–(S2) in Fig. 3. The latter suggests that the ability of the network to learn the set of training patterns is independent of the version of the model used. Thus, the conclusions drawn from the analysis of (S1)–(S2) can be applied to the alternative form (S7)–(S8).

In Fig. S2(a)–(c), various stages of learning are illustrated by analogy with Fig. 3(a)–(c). One can follow the development of memories in the NN as time goes by and the same vectors are applied to the system again and again. Note, that although the numbers of memories formed by the end of learning in two models appear very similar, the two versions of the model do not learn in the same way. For example, attractors at  $t=2000$  are different in Figs. 3(c) and S2(c). Thus, each individual memory may be formed at a different time depending on the version of the model being used.

Next, using the same methods as those presented in Sec. VI of the main paper, we visualise the basins of attraction of some attractors formed at the end of learning by the NN (S7)–(S8). We consider an intersection of the 81-dimensional phase space with a plane defined by the set of equations  $x_3=x_3^*$ ,  $x_4=0, \dots, x_{81}=0$ , where  $x_3^*$  takes the values we choose. As a result, we obtain a two-dimensional cross-section on  $(x_1, x_2)$ -plane. Twelve such cross-sections, corresponding to twelve different values of  $x_3^*$ , are presented in Fig. S3. The chosen values of  $x_3^*$  are uniformly spaced and identical to those illustrated in Fig. 13 for the basins of the model (S1)–(S2), as indicated above each panel in Fig. S3. Also, on each panel one can see projections of all attractors present in (S7)–(S8) at the end of learning at  $t=6000$  (coloured filled rectangles), whose colours match those of their basins.

As Fig. S3 illustrates, the cross-sections of the attractor basins hold high resemblance to those in Fig. 13 (albeit with an alternative colour coding) both in terms of their number and shape. This highlights the fact that the ability of the Hopfield network to memorise patterns appears to be independent of the specific choice of the model, and the memories formed are identical in both cases, at least in a qualitative sense.

Bifurcation mechanisms responsible for the formation and destruction of memories can also be shown to be identical in both NNs, however, the respective results are not presented here.

To finalise the comparison between learning with two different forms of the Hopfield NN, by analogy with Fig. 14, in Fig. S4 we illustrate the nature of the boundaries of attractor basins formed at the end of their learning from the same training Set 1. These boundaries are formed by the stable manifolds of saddle fixed points with exactly one positive eigen-

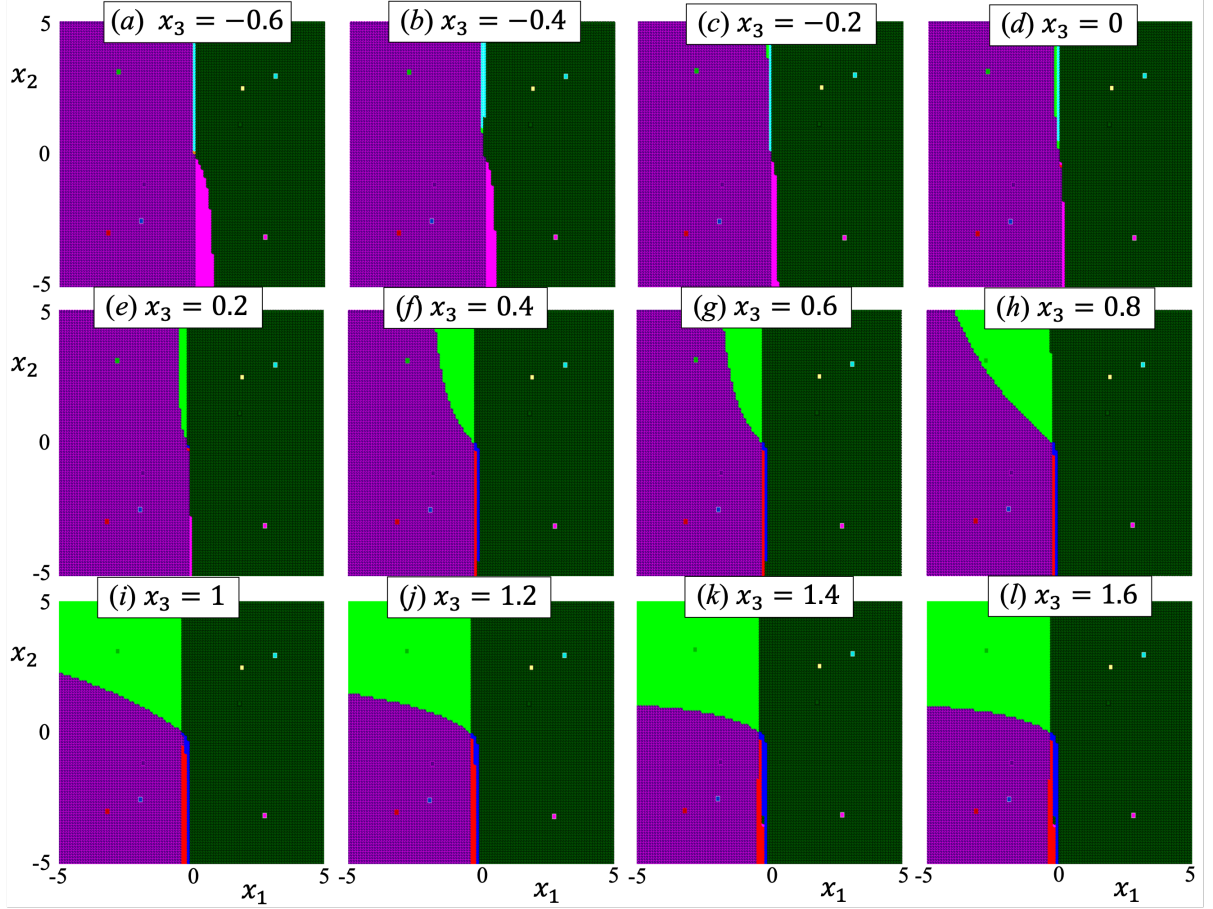

FIG. S3. Attractor basins (shaded regions in various colours) at the end of learning in Hopfield NN in alternative form (S7)–(S8) with  $N=81$ ,  $g=0.3$ ,  $B=300$ ,  $A=30$ . Points in various colours show projections of attractors, some of which represent spurious memories (compare with Fig. S2(d)). Being volumes in 81-dimensional space, the basins (a)–(l) are shown as cross-sections by twelve different planes (same as in Fig. 13 of the main paper) defined as  $x_3=x_3^*$ ,  $x_i=0$ ,  $i=4, \dots, 81$ , where  $x_3^*$  takes values from  $[-0.6, 1.6]$  (see values in each panel).

value.

In Fig. S4, four additional distinct cross-sections are shown of the same attractor basins as the ones illustrated in Fig. S3. Here, to obtain different panels, different secant planes were used. Namely, the secant planes are defined as  $x_i=s_i^m$ ,  $i=3, \dots, 81$ , where  $s_i^m$  is the  $i^{\text{th}}$  coordinate of the  $m^{\text{th}}$  saddle point with one positive eigenvalue (white diamond). We consider four different saddle points, so  $m=1, \dots, 4$ . Thus, different secant planes go through different saddle points. Therefore, different cross-sections in Fig. S4(a)–(c) contain different saddle points shown as white diamonds.

Fig. S4 illustrates that, as in Fig. 14 of the main paper, the saddle points lie exactly on the boundaries between the basins of attraction. The latter fact verifies that these boundaries are indeed formed by the stable manifolds of the respective saddle points.

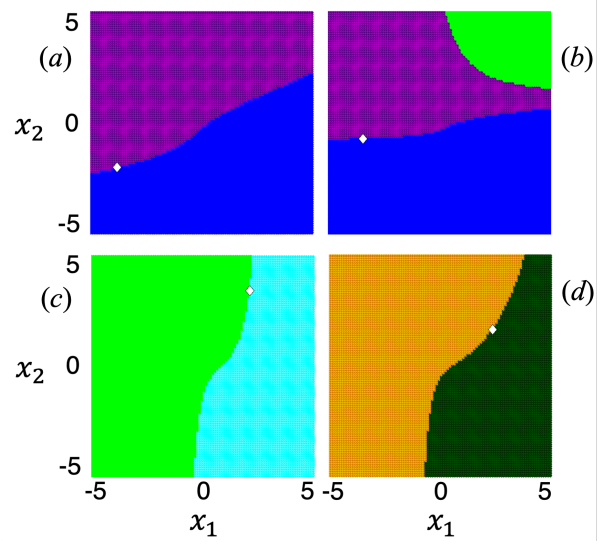

FIG. S4. Attractor basins (shaded regions in various colours) at the end of learning in Hopfield NN in an alternative form (S7)–(S8) with  $N=81$ . Basin boundaries are formed by stable 80-dimensional manifolds of saddle fixed points with one positive eigenvalue. Basins are shown as cross-sections with secant planes, each going through one of four different saddles (white diamonds). See text for details.

## S-IV. APPENDIX OF TABLES

| $I_i^k$ | $i$ | Set 1: $k = 1 \dots 6$ |    |    |    |    |    | Set 2: $k = 1 \dots 6$ |    |    |    |    |    |
|---------|-----|------------------------|----|----|----|----|----|------------------------|----|----|----|----|----|
|         |     | 1                      | 2  | 3  | 4  | 5  | 6  | 1                      | 2  | 3  | 4  | 5  | 6  |
|         | 1   | -1                     | 1  | -1 | -1 | -1 | -1 | -1                     | 1  | 1  | -1 | 1  | -1 |
|         | 2   | -1                     | 1  | 1  | -1 | 1  | 1  | -1                     | -1 | -1 | 1  | 1  | -1 |
|         | 3   | 1                      | -1 | -1 | -1 | -1 | 1  | -1                     | -1 | -1 | -1 | -1 | -1 |
|         | 4   | 1                      | -1 | 1  | -1 | -1 | -1 | -1                     | 1  | 1  | -1 | 1  | 1  |
|         | 5   | -1                     | -1 | 1  | -1 | -1 | -1 | -1                     | 1  | -1 | -1 | 1  | -1 |
|         | 6   | -1                     | 1  | -1 | 1  | 1  | 1  | 1                      | -1 | 1  | -1 | 1  | 1  |
|         | 7   | -1                     | -1 | 1  | -1 | -1 | 1  | -1                     | 1  | -1 | -1 | 1  | 1  |
|         | 8   | -1                     | -1 | 1  | 1  | -1 | 1  | -1                     | 1  | -1 | -1 | 1  | 1  |
|         | 9   | 1                      | 1  | 1  | -1 | 1  | -1 | 1                      | -1 | -1 | -1 | 1  | -1 |
|         | 10  | -1                     | -1 | -1 | 1  | 1  | -1 | -1                     | 1  | 1  | -1 | -1 | -1 |
|         | 11  | 1                      | -1 | -1 | 1  | 1  | 1  | 1                      | -1 | -1 | 1  | -1 | 1  |
|         | 12  | -1                     | 1  | -1 | -1 | -1 | 1  | -1                     | 1  | -1 | 1  | -1 | -1 |
|         | 13  | -1                     | -1 | 1  | 1  | -1 | -1 | 1                      | -1 | -1 | 1  | 1  | 1  |
|         | 14  | -1                     | -1 | 1  | -1 | 1  | -1 | -1                     | 1  | 1  | 1  | -1 | -1 |
|         | 15  | 1                      | -1 | -1 | 1  | 1  | -1 | -1                     | -1 | 1  | 1  | -1 | -1 |
|         | 16  | -1                     | -1 | 1  | -1 | -1 | -1 | 1                      | 1  | 1  | -1 | -1 | -1 |
|         | 17  | -1                     | 1  | -1 | 1  | 1  | -1 | 1                      | -1 | 1  | -1 | 1  | 1  |
|         | 18  | 1                      | -1 | -1 | 1  | 1  | -1 | 1                      | 1  | 1  | -1 | 1  | 1  |
|         | 19  | 1                      | 1  | 1  | 1  | 1  | -1 | -1                     | -1 | 1  | -1 | 1  | 1  |
|         | 20  | 1                      | 1  | 1  | -1 | -1 | -1 | 1                      | -1 | 1  | -1 | 1  | -1 |
|         | 21  | -1                     | -1 | 1  | -1 | 1  | 1  | -1                     | -1 | 1  | -1 | 1  | -1 |
|         | 22  | 1                      | 1  | -1 | 1  | -1 | 1  | -1                     | -1 | 1  | 1  | 1  | -1 |
|         | 23  | -1                     | -1 | 1  | -1 | -1 | 1  | -1                     | 1  | 1  | -1 | -1 | -1 |
|         | 24  | 1                      | -1 | 1  | 1  | 1  | 1  | -1                     | 1  | -1 | 1  | -1 | -1 |
|         | 25  | -1                     | -1 | 1  | -1 | -1 | -1 | -1                     | -1 | 1  | 1  | -1 | -1 |
|         | 26  | 1                      | 1  | -1 | 1  | 1  | -1 | 1                      | 1  | -1 | -1 | 1  | -1 |
|         | 27  | -1                     | -1 | -1 | -1 | 1  | 1  | -1                     | -1 | 1  | 1  | 1  | -1 |
|         | 28  | -1                     | 1  | 1  | -1 | -1 | -1 | -1                     | 1  | -1 | -1 | -1 | -1 |
|         | 29  | -1                     | -1 | -1 | -1 | -1 | 1  | -1                     | 1  | 1  | -1 | 1  | -1 |
|         | 30  | -1                     | -1 | -1 | -1 | 1  | -1 | 1                      | -1 | 1  | -1 | 1  | 1  |
|         | 31  | 1                      | -1 | -1 | 1  | -1 | 1  | -1                     | -1 | -1 | 1  | -1 | -1 |
|         | 32  | -1                     | 1  | 1  | 1  | -1 | -1 | 1                      | -1 | -1 | 1  | 1  | 1  |
|         | 33  | -1                     | -1 | 1  | -1 | 1  | -1 | -1                     | 1  | -1 | 1  | -1 | 1  |
|         | 34  | -1                     | 1  | -1 | 1  | -1 | 1  | 1                      | 1  | 1  | 1  | -1 | -1 |
|         | 35  | 1                      | 1  | -1 | 1  | 1  | 1  | 1                      | 1  | 1  | 1  | -1 | 1  |
|         | 36  | 1                      | -1 | -1 | 1  | 1  | 1  | 1                      | -1 | -1 | -1 | -1 | -1 |
|         | 37  | -1                     | 1  | 1  | 1  | 1  | 1  | 1                      | 1  | -1 | -1 | -1 | -1 |
|         | 38  | -1                     | -1 | 1  | -1 | -1 | 1  | -1                     | 1  | -1 | 1  | -1 | -1 |
|         | 39  | -1                     | 1  | -1 | 1  | -1 | 1  | 1                      | -1 | -1 | -1 | -1 | -1 |
|         | 40  | -1                     | 1  | 1  | 1  | 1  | -1 | 1                      | 1  | -1 | -1 | 1  | 1  |
|         | 41  | 1                      | 1  | -1 | 1  | 1  | 1  | -1                     | 1  | 1  | -1 | 1  | -1 |

TABLE S1. First part of Table showing two distinct sets, Set 1 and Set 2, of six stimulus vectors  $\mathbf{I}^k$ ,  $k=1 \dots 6$ , used to train the network (S1)–(S2) (also (1)–(2)) with  $N=81$ . Here, components  $I_i^k$  are given for  $i=1, \dots, 41$ .

| $I_i^k$ | Set 1: $k = 1 \dots 6$ |    |    |    |    |    | Set 2: $k = 1 \dots 6$ |    |    |    |    |    |
|---------|------------------------|----|----|----|----|----|------------------------|----|----|----|----|----|
|         |                        |    |    |    |    |    |                        |    |    |    |    |    |
| 42      | -1                     | 1  | -1 | 1  | 1  | 1  | 1                      | 1  | -1 | -1 | 1  | 1  |
| 43      | -1                     | -1 | -1 | 1  | 1  | 1  | -1                     | 1  | -1 | -1 | 1  | 1  |
| 44      | 1                      | 1  | 1  | 1  | 1  | 1  | -1                     | 1  | -1 | -1 | 1  | 1  |
| 45      | -1                     | 1  | 1  | -1 | 1  | 1  | 1                      | 1  | -1 | 1  | 1  | 1  |
| 46      | 1                      | 1  | -1 | 1  | -1 | 1  | 1                      | -1 | 1  | -1 | -1 | -1 |
| 47      | 1                      | 1  | -1 | -1 | -1 | 1  | 1                      | -1 | 1  | -1 | 1  | -1 |
| 48      | -1                     | 1  | -1 | -1 | 1  | -1 | 1                      | 1  | 1  | -1 | 1  | -1 |
| 49      | -1                     | -1 | -1 | -1 | 1  | -1 | 1                      | -1 | -1 | 1  | -1 | 1  |
| 50      | -1                     | -1 | -1 | -1 | -1 | -1 | -1                     | -1 | -1 | -1 | -1 | 1  |
| 51      | -1                     | 1  | -1 | -1 | 1  | -1 | -1                     | 1  | 1  | 1  | -1 | 1  |
| 52      | 1                      | -1 | 1  | -1 | 1  | -1 | -1                     | -1 | 1  | -1 | -1 | -1 |
| 53      | 1                      | -1 | -1 | 1  | 1  | -1 | 1                      | -1 | 1  | 1  | -1 | 1  |
| 54      | 1                      | 1  | -1 | 1  | 1  | -1 | -1                     | 1  | 1  | 1  | -1 | -1 |
| 55      | 1                      | -1 | 1  | -1 | 1  | 1  | -1                     | 1  | -1 | 1  | -1 | 1  |
| 56      | 1                      | 1  | -1 | 1  | 1  | -1 | 1                      | -1 | -1 | -1 | -1 | 1  |
| 57      | 1                      | 1  | -1 | -1 | -1 | -1 | 1                      | 1  | -1 | 1  | 1  | -1 |
| 58      | -1                     | -1 | -1 | 1  | -1 | -1 | -1                     | -1 | -1 | 1  | -1 | 1  |
| 59      | -1                     | 1  | 1  | 1  | -1 | 1  | 1                      | -1 | -1 | 1  | 1  | -1 |
| 60      | 1                      | -1 | -1 | 1  | -1 | -1 | -1                     | 1  | -1 | -1 | 1  | -1 |
| 61      | 1                      | 1  | -1 | -1 | 1  | 1  | 1                      | 1  | 1  | 1  | 1  | 1  |
| 62      | -1                     | -1 | 1  | 1  | -1 | -1 | -1                     | -1 | 1  | -1 | -1 | 1  |
| 63      | 1                      | -1 | 1  | -1 | -1 | -1 | 1                      | -1 | -1 | -1 | -1 | -1 |
| 64      | -1                     | -1 | -1 | -1 | -1 | 1  | 1                      | -1 | -1 | 1  | -1 | 1  |
| 65      | 1                      | 1  | 1  | -1 | 1  | 1  | -1                     | 1  | 1  | -1 | 1  | 1  |
| 66      | 1                      | -1 | -1 | 1  | 1  | -1 | 1                      | -1 | -1 | 1  | -1 | -1 |
| 67      | 1                      | 1  | 1  | -1 | 1  | -1 | -1                     | 1  | -1 | 1  | 1  | -1 |
| 68      | -1                     | -1 | 1  | -1 | -1 | -1 | -1                     | -1 | -1 | -1 | -1 | 1  |
| 69      | 1                      | -1 | 1  | 1  | -1 | -1 | 1                      | -1 | -1 | -1 | 1  | -1 |
| 70      | 1                      | 1  | -1 | 1  | -1 | -1 | 1                      | 1  | 1  | 1  | -1 | 1  |
| 71      | 1                      | -1 | 1  | -1 | 1  | 1  | 1                      | -1 | -1 | 1  | 1  | 1  |
| 72      | -1                     | -1 | 1  | 1  | 1  | 1  | 1                      | -1 | -1 | -1 | 1  | 1  |
| 73      | -1                     | -1 | 1  | -1 | -1 | -1 | 1                      | 1  | -1 | -1 | -1 | 1  |
| 74      | -1                     | 1  | -1 | 1  | 1  | 1  | -1                     | 1  | -1 | 1  | 1  | -1 |
| 75      | -1                     | 1  | -1 | -1 | -1 | -1 | -1                     | 1  | -1 | -1 | -1 | -1 |
| 76      | 1                      | 1  | -1 | -1 | -1 | 1  | -1                     | -1 | 1  | 1  | -1 | -1 |
| 77      | 1                      | 1  | 1  | 1  | -1 | -1 | -1                     | 1  | -1 | -1 | -1 | -1 |
| 78      | -1                     | 1  | 1  | -1 | 1  | 1  | 1                      | -1 | 1  | 1  | 1  | -1 |
| 79      | 1                      | -1 | 1  | -1 | -1 | 1  | -1                     | -1 | 1  | 1  | -1 | 1  |
| 80      | -1                     | -1 | -1 | -1 | -1 | -1 | 1                      | 1  | 1  | -1 | 1  | 1  |
| 81      | -1                     | -1 | -1 | 1  | 1  | 1  | 1                      | -1 | -1 | -1 | -1 | -1 |

TABLE S2. Second part of Table showing two distinct sets, Set 1 and Set 2, of six stimulus vectors  $\mathbf{I}^k$ ,  $k=1 \dots 6$ , used to train the network (S1)–(S2) (also (1)–(2)) with  $N=81$ . Here, components  $I_i^k$  are given for  $i=42, \dots, 81$ .

| $I_i^k$ |   | <b>Set 1: <math>k=1 \dots 3</math></b> |    |    |
|---------|---|----------------------------------------|----|----|
| $i$     | 1 | 1                                      | -1 | -1 |
|         | 2 | -1                                     | -1 | 1  |
|         | 3 | -1                                     | -1 | -1 |

TABLE S3. Set of three stimulus vectors  $\mathbf{I}^k$ ,  $k=1 \dots 3$ , used to train the network (S1)–(S2) (also (1)–(2)) with  $N=3$ .

[S1] D. Dong and J. Hopfield, “Dynamic properties of neural networks with adapting synapses,” *Network: Computation in Neural Systems* **3**, 267–283 (1992).
